# Supplementary material for: Super-resolution Localization of Nitrogen Vacancy Centers in Diamond with Quantum Controlled Photoswitching
Source: arXiv:2008.01970 source file (2020-08-05)
Supplement: Supplementary file 1 [file Supplementary_Materials.pdf]

Supplementary Materials for

"Super-resolution Localization of Nitrogen Vacancy Centers with Quantum Controlled Photoswitching"

**Supplementary Note 1. The minimum resolution of gradient quantum control**

In the main text, we demonstrate the localization of two nearby NV centers separated by 266 nm with quantum controlled photoswitching (QCP). The ultimate capability of localization based on our approach mostly depends on the resolution of gradient quantum control. From the results of magnetic field gradient (MFG) calibration (Fig. S1), where the maximum MFG at NV A is 7.35 G/μm under 10 mA current, we simulate the ultimate resolution of QCP (Fig. S2) under the assumption that the two adjacent NV centers hold the same coherent property. Fig. S2a elucidates the simulation result under the precession time at $\tau$ = 160 μs. The three solid black curves denote the corresponding condition (the accumulated phase differences at $\pi$, $3\pi$ and $5\pi$) to manipulate these two NV centers into $|0\rangle\otimes|1\rangle$ or $|1\rangle\otimes|0\rangle$ state alternatively. From the lowermost solid black curve we can acquire that the minimum resolution of QCP is ~0.15 nm. The detailed results of ultimate resolution of QCP at 0.15 nm are plotted in Fig. S2b and c. At the maximum MFG, the quantum states of the two NV centers evolve into our desired $|1\rangle\otimes|0\rangle$ or $|0\rangle\otimes|1\rangle$ states alternatively at close to 10 mA current magnitude. The dashed lines in Fig. S2c correspond to $|1\rangle\otimes|0\rangle$ and $|0\rangle\otimes|1\rangle$ state, where the current values are 9.87 and 9.95 mA, respectively. Based on the Fourier space image results in Fig. S2b, we can obtain the real space image (Fig. S2d) with the pixel resolution at 0.3 nm, which is two times larger than our resolution of QCP. Moreover, it is difficult for us to distinguish the two NV centers clearly.

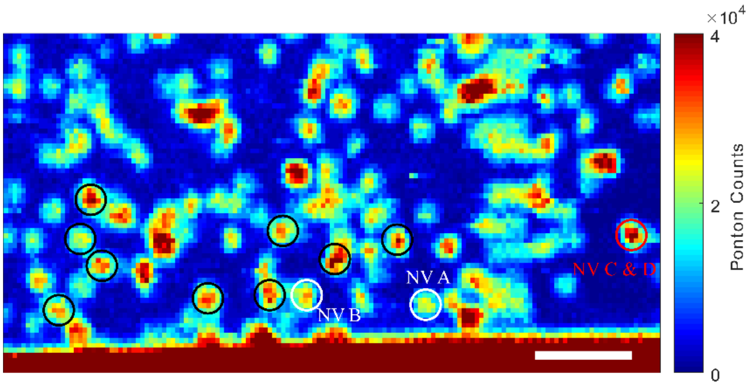


FIG. S1. The confocal intensity map of the selected NV centers for MFG calibration (marked by the black and white circles). The red line at the bottom of the map is the microwire of MFG. Scale bar: 2 μm.

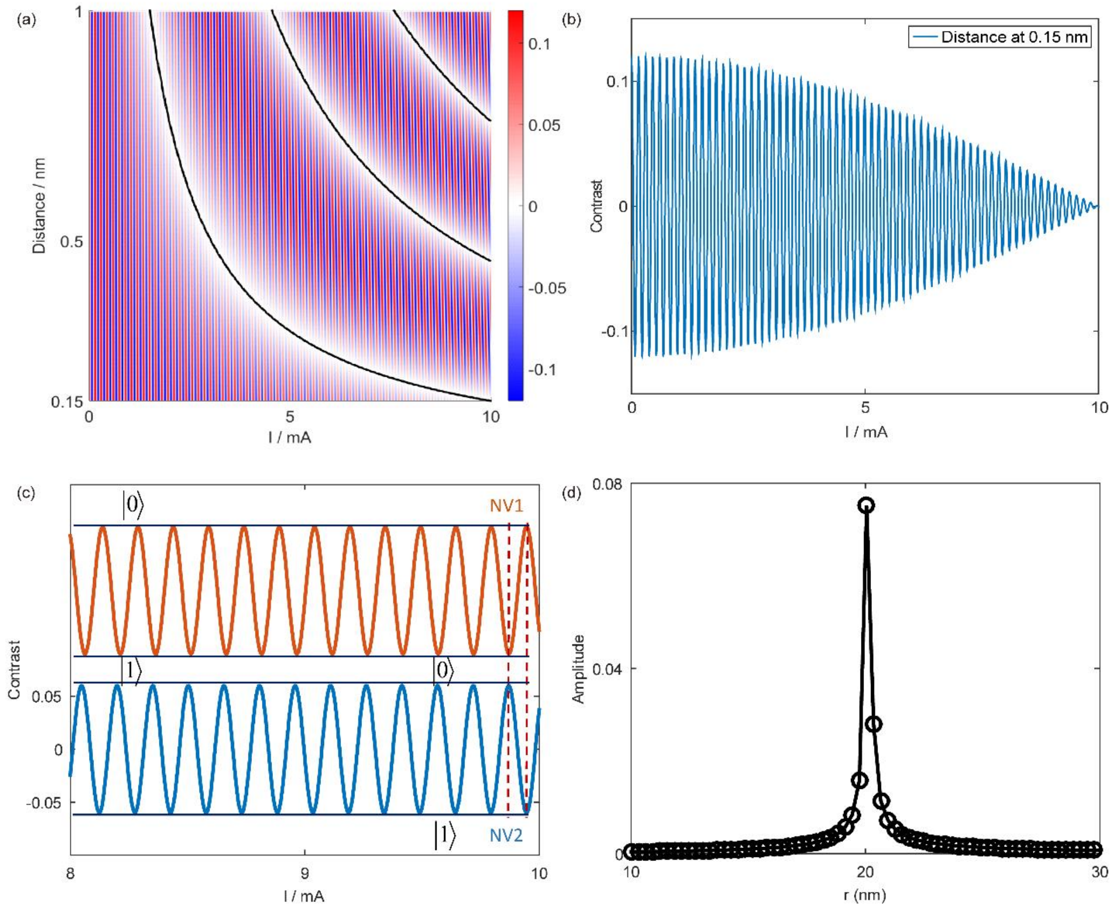


FIG. S2. The simulation results of the ultimate resolution of QCP. (a) The ultimate resolution of QCP at the maximum MFG. The vertical axis represents the distance between the two nearby NV centers. (b) The Fourier space image on the occasion of QCP resolution at 0.15 nm. (c) Illustration of the state evolution of each NV center decomposed from (b). (d) Real space image obtained from Fast Fourier Transformation of (b).

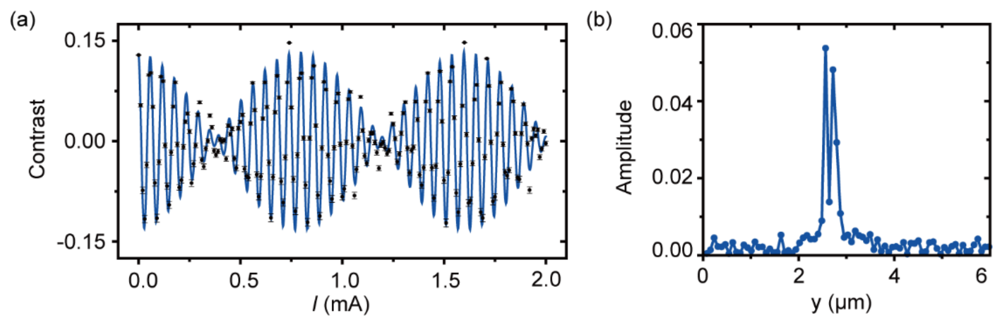


FIG. S3. The one dimensional Fast Fourier Transform (FFT) magnetic imaging of NV C & D. (a) The raw data of k space. (b) FFT of (a) to real space. The two peaks separating by 151 nm reveals the distance of the two NV centers alongside y axis. This

is in good agreement with the distance of 156 nm taken from the super-resolution optical imaging in Fig. 4 in the main text.

**Supplementary Note 2. Coherent control and qubit operation on NV centers**

In Fig.1 & 3 of the main text, the quantum states of NV C and NV D are manipulated to |1> or |0> by the quantum phase encoding. Furthermore, by varying the pulsed gradient magnetic field and the evolution time, each qubit could be quantum manipulated and readout individually on demand. Here are examples of experiments on two NV centers (NV C & D) and simulations on coupled NV centers:

(1) The Rabi Oscillation of NV C & D:

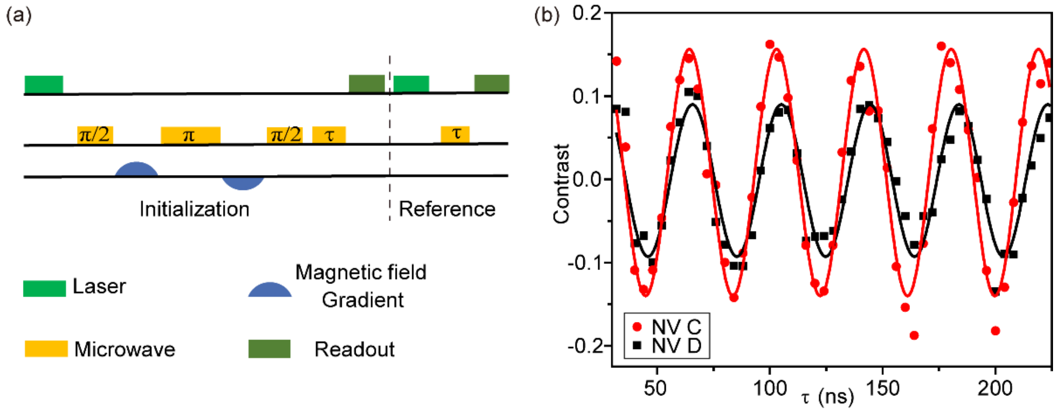


FIG. S4. The Rabi oscillation of NV C & D. (a) The respective Rabi pulse sequence for the individual NV center. (b) The results of each NV center's Rabi oscillation. From the cosine function fitting results, the π pulses for NV C and NV D are 19.4 ns and 19.7 ns, respectively.

(2) The measurement of free induction decay of NV C & D:

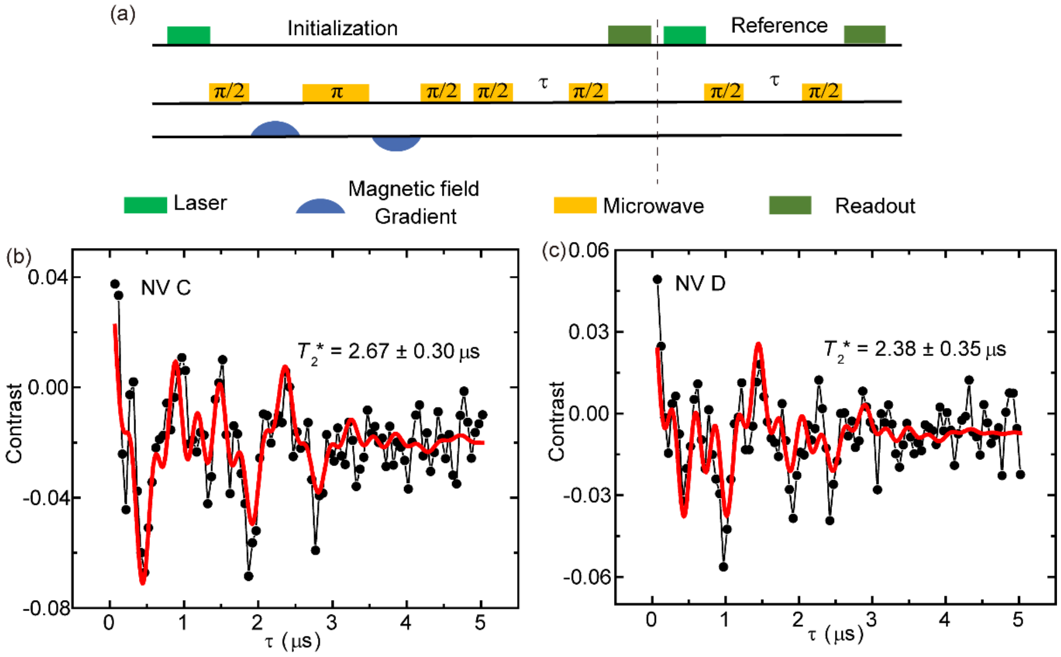

FIG. S5. The Ramsey experiment of NV C & D. (a) The pulse sequence for the FID measurement of each NV center. (b), (c) The experimental results of each NV center's FID measurement. The red solid curves are the fitting results with the fitting function of $\sum_{i=1}^{3} A_i \bullet \cos(2\pi f_i \tau)$.

From the results of Fig. S5, we can site-selective address each NV center's Ramsey measurement. The $T_2^*$ for NV C and NV D are 2.67 μs and 2.38 μs, respectively.

(3) Single qubit phase gate. The phase accumulated on the *j*th qubit of uncoupled NV centers is written by:

$$\varphi_j = \gamma\tau \int_0^\tau G\left(r_j, t, I\right) r_j \, dt$$

where $\gamma$ is the gyromagnetic ratio, $\tau$ is the total evolution time, $G$ is the magnetic field gradient, $r$ is the position of NV center, and $I$ is the current in the gradient microwire. The final state is

$$\Psi_j = \cos\varphi_j \left|0\right\rangle + i\sin\varphi_j \left|1\right\rangle$$

The NOT gate on the *j*th qubit can be expressed by $U(\varphi_j = \pi)$.

Owing to lacking of suitable sample containing two or three coupled NV centers below 10nm, we add a calculation on two coupled NV centers to prove that coherent control or qubit operations can be performed using this imaging technique. Given that the two coupled NV centers ($NV_1$ and $NV_2$) are away from 10nm, the spin Hamiltonian of this system for $NV_1$ (S=1) can be written as

$$H_1 = \gamma_e G(r_1, I) r_1 S_1 + S_1 \bullet A \bullet S_2,$$

where $\gamma_e$ is the electron gyromagentic ratio, $G(r_1, I)$ is the magnetic field gradient, $r_1$ is the relative location of $NV_1$, $I$ is the current in the gradient microwire, and A is the hyperfine constant, respectively. Under the secular approximation, the transverse components of the hyperfine constant can be neglected, so the hyperfine constant can be simplified as $A=A_{zz}=a$. When this system evolves under spin-echo phase encoding pulse sequence (Fig. S6a), the first π/2 pulse prepares the spin state of $NV_1$ into quantum superposition state $(|0\rangle + |1\rangle)/\sqrt{2}$. Then during the evolution time, there is an accumulated phase on the $NV_1$ center $\varphi_1=(\gamma_e G(r_1, I)r_1+a)\tau$, so the detected signal for $NV_1$ is $S_1= C_1\cos\varphi_1$, where $C_1$ is the normalized fluorescence intensity, and $\tau$ is the interrogation time. Similarly, the detected signal for $NV_2$ is $S_2= C_2\cos\varphi_2$, where $\varphi_2=(\gamma_e G(r_2, I)r_2+a)\tau$. Then the total signal for this system can be written as

$$S_{tot}= S_1+S_2= C_1\cos\varphi_1+ C_2\cos\varphi_2.$$

When $\varphi_2-\varphi_1=\pi/2, \pi, 3\pi/2, 2\pi$ and $\varphi_1=2n\pi$, we can perform the corresponding qubit operation (π/2, π, 3π/2, 2π phase gates) on the $NV_2$ without any effect on $NV_1$. From

the simulation result of Fig. S6b, by tuning the magnetic gradient field sent through the microwire, single qubit phase gate on the coupled NV centers system can be achieved using our imaging technique.

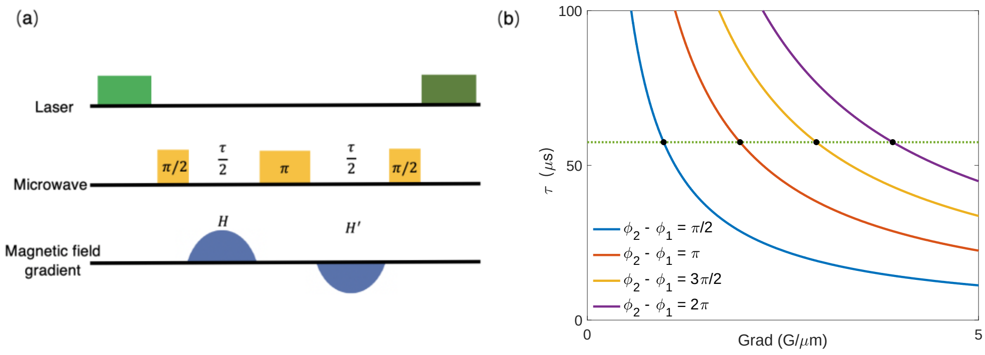


FIG. S6. The simulation result of single qubit phase gate on two coupled NV centers away from 10nm. The solid lines from left to right are $\varphi_2$-$\varphi_1$=π/2, π, 3π/2, 2π, respectively. While the black dots from left to right are $\varphi_1=2n\pi$ ($n$=8, 16, 24, 32) for $NV_1$. Therefore, these four points represent π/2, π, 3π/2, 2π qubit operations performed on the $NV_2$ while $NV_1$ is not affected, respectively.
